# Supplementary material for: U-Boost NAS: Utilization-Boosted Differentiable Neural Architecture Search
Source: arXiv:2203.12412 source file (2022-03-23)
Supplement: Supplementary file 1 [file placeholder.tex]

\section{Placeholder}

\begin{itemize}
    \item add figures of micro arch search space for different util coeefs, hw models
    \item learning curves
    \item add table with findings per hw model and per latency coeff
    \item cells for imagenet
\end{itemize}
